# Supplementary material for: Remote Entanglement by Coherent Multiplication of Concurrent Quantum Signals
Source: arXiv:1505.01178 source file (2015-09-10)
Supplement: Supplementary file 1 [file Supplement.pdf]

# Supplementary Material for
# Remote Entanglement by Coherent Multiplication of Concurrent Quantum Signals

Ananda Roy,[1,*] Liang Jiang,[1] A. Douglas Stone,[1] and Michel Devoret[1]

[1]*Department of Applied Physics, Yale University, PO BOX 208284, New Haven, CT 06511*

## SCHEMATIC OF EXPERIMENTAL SETUP

Here, we show a more detailed schematic of the proposed experimental setup (Fig. 1). Two transmon qubits, Alice and Bob, are initialized in their respective $(|g\rangle + |e\rangle)/\sqrt{2}$ states. They are dispersively coupled to auxiliary cavity modes $\mathbf{A}, \mathbf{B}$ respectively. The output from the cavity modes $\mathbf{A}, \mathbf{B}$, after propagation on transmission lines, exicte the high-Q modes $\mathbf{a}, \mathbf{b}$ respectively. The modes $\mathbf{a}, \mathbf{b}$ and $\mathbf{c}$ participate in a three-wave mixing interaction, in presence of a stiff, off-resonant pump through the Josephson Four Wave Mixer (see below). The three cavities a,b,c, together with the Josephson Four Wave Mixer, comprise the Josephson Parametric Multiplier (JPM). The outputs of each of the cavities a,b,c are monitored with homodyne detection, denoted respectively by $\mathrm{HD_a}, \mathrm{HD_b}, \mathrm{HD_c}$.

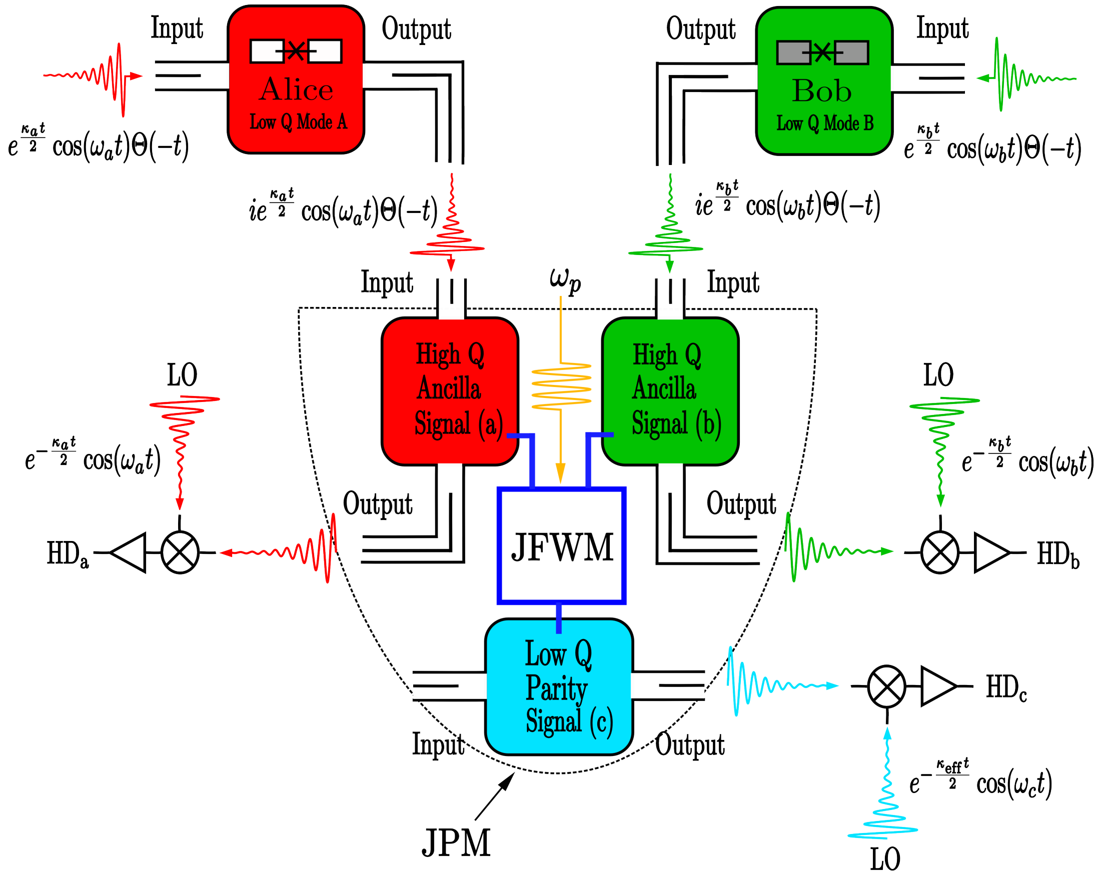


FIG. 1. (color online) Schematic of experimental setup for remote entanglement protocol. Two transmon qubits, Alice and Bob, are off-resonantly coupled to auxiliary resonator modes (frequencies) $\mathbf{A}(\omega_a)$ and $\mathbf{B}(\omega_b)$. The outputs of the modes $\mathbf{A}$ and $\mathbf{B}$, after propagating through transmission lines, act as inputs to the $\mathbf{a}$ and $\mathbf{b}$ modes respectively. The modes $\mathbf{a}(\omega_a), \mathbf{b}(\omega_b)$ and $\mathbf{c}(\omega_c)$ participate in a non-linear, three-wave interaction $\mathbf{H}_{\mathrm{int}}/\hbar = ige^{-i\omega_p t}\mathbf{abc}^\dagger + \mathrm{h.c.}$, conditioned on the presence of an off-resonant, stiff pump (in orange) at frequency $\omega_p = \omega_c - \omega_a - \omega_b$. This nonlinear mode mixing arises out of the Josephson Four Wave Mixer (JFWM). The JFWM, together with the resonators of the three interacting modes, comprise the JPM of Fig. (1) in the main text. The outputs of each of the modes $\mathbf{a}, \mathbf{b}$ and $\mathbf{c}$ are monitored with homodyne detection, denoted by $\mathrm{HD_a}, \mathrm{HD_b}$ and $\mathrm{HD_c}$, respectively. (Inset) The JFWM has four nominally identical Josephson junctions and has four mutually orthogonal interacting normal (electrical) modes, respectively corresponding to the modes $\mathbf{a}, \mathbf{b}, \mathbf{c}$ and the stiff, off-resonant pump (see below). The Josephson nonlinearity, together with the off-resonant pump, gives rise to the desired three-wave interaction given by $\mathbf{H}_{\mathrm{int}}$ under rotating wave approximation.

## TEMPORAL PROFILE CALCULATION

We show our computation for the dispersive phase shift gathered from dispersive interaction of the propagating ancilla signal mode a with Alice's qubit. For brevity, we will compute for the case when the ancilla signal (a) is reflected

off Alice's qubit and proceeds on to be incident on the JPM. One can obtain similar results for the transmission case. The complete cavity-qubit Hamiltonian for the cavity mode $A$ dispersively coupled to Alice's qubit can be written as:

$$\mathbf{H}_{\text{A}-\text{Alice}} = \hbar\omega_a \mathbf{A}^\dagger \mathbf{A} + \hbar\omega_q \sigma_z + \chi \mathbf{A}^\dagger \mathbf{A} \sigma_z, \tag{1}$$

where $\omega_{a(q)}$ is the frequency of the cavity (qubit) and $\chi$ is the strength of the dispersive interaction between the two. Going to the rotating frame of the cavity at its resonant frequency and that of the qubit, the effective Hamiltonian becomes:

$$\mathbf{H}_{\text{disp}} = \chi \mathbf{A}^\dagger \mathbf{A} \sigma_z. \tag{2}$$

We will consider the case when the cavity is excited resonantly. Then, the Langevin equations of motion for the qubit-cavity system (neglecting the dissipation channels of the qubit) can be written as:

$$\frac{d\mathbf{A}}{dt} = -\frac{\kappa_A}{2}\mathbf{A} - i\chi \mathbf{A}\sigma_z + \sqrt{\kappa_A}\mathbf{A}^{\text{in}}, \qquad \mathbf{A}^{\text{in}} + \mathbf{A}^{\text{out}} = \sqrt{\kappa_A}\mathbf{A}, \tag{3}$$

or equivalently,

$$\frac{d\mathbf{A}^{\text{out}}}{dt} + \frac{\kappa_A}{2}\mathbf{A}^{\text{out}} + i\chi\sigma_z \mathbf{A}^{\text{out}} = -\frac{d\mathbf{A}^{\text{in}}}{dt} + \frac{\kappa_A}{2}\mathbf{A}^{\text{in}} - i\chi\sigma_z \mathbf{A}^{\text{in}}, \tag{4}$$

where $\kappa_A$ is the cavity decay rate for the mode $\mathbf{A}$.

Denoting the output field amplitude when the qubit is in the excited (ground) state by $A^{\text{out}}_{e(g)}$, we can write the equations governing the dynamics of each of them:

$$\frac{dA^{\text{out}}_e}{dt} + \frac{\kappa_A}{2}A^{\text{out}}_e + i\chi A^{\text{out}}_e = -\frac{dA^{\text{in}}}{dt} + \frac{\kappa_A}{2}A^{\text{in}} - i\chi A^{\text{in}}, \tag{5}$$

$$\frac{dA^{\text{out}}_g}{dt} + \frac{\kappa_A}{2}A^{\text{out}}_g - i\chi A^{\text{out}}_g = -\frac{dA^{\text{in}}}{dt} + \frac{\kappa_A}{2}A^{\text{in}} + i\chi A^{\text{in}}. \tag{6}$$

Without loss of generality, we consider the case when incident field amplitude $A^{\text{in}} = A^{\text{in}*}$, in which case $A^{\text{out}}_g = A^{\text{out}*}_e$ and thus, Eqn. (5) and Eqn. (6) are identical to each other. Similar computations can be performed for $A^{\text{in}} \notin \Re$.

Let us define: $A^{\text{out}}_g = x + iy$, implying $A^{\text{out}}_e = x - iy$. Adding and subtracting Eqns. (5) and (6), we arrive at:

$$\frac{dx}{dt} + \frac{\kappa_A}{2}x + \chi y = -\frac{dA^{\text{in}}}{dt} + \frac{\kappa_A}{2}A^{\text{in}} \tag{7}$$

$$\frac{dy}{dt} + \frac{\kappa_A}{2}y - \chi x = \chi A^{\text{in}}. \tag{8}$$

We will look for solutions of $x(t), y(t)$ for $A^{\text{in}}(t) = \sqrt{\kappa_a}e^{\kappa_a t/2}\theta(-t)$, where $\kappa_a$ is the cavity decay rate of the high-Q signal mode of the JPM.

Solving Eqns. (7) and (8), we arrive at:

$$x(t) = \frac{\sqrt{\kappa_a}}{(\kappa_a+\kappa_A)^2 + 4\chi^2}\Big[(\kappa_A^2 - \kappa_a^2 - 4\chi^2)e^{\kappa_a t/2}\theta(-t) + \theta(t)e^{-\kappa_A t/2}\Big\{2\kappa_A(\kappa_A+\kappa_a)\cos(\chi t) - 4\chi\kappa_A\sin(\chi t)\Big\}\Big] \tag{9}$$

$$y(t) = \frac{2\sqrt{\kappa_a}\kappa_A}{(\kappa_a+\kappa_A)^2 + 4\chi^2}\Big[2\chi e^{\kappa_a t/2}\theta(-t) + \theta(t)e^{-\kappa_A t/2}\Big\{2\chi\cos(\chi t) + (\kappa_A+\kappa_a)\sin(\chi t)\Big\}\Big]. \tag{10}$$

We require $\kappa_a \ll \kappa_A = 2\chi$, whence:

$$x(t) = \sqrt{\kappa_a}\theta(t)e^{-\kappa_A t/2}\Big\{\cos(\kappa_A t/2) - \sin(\kappa_A t/2)\Big\} \tag{11}$$

$$y(t) = \sqrt{\kappa_a}e^{\kappa_a t/2}\theta(-t) + \sqrt{\kappa_a}\theta(t)e^{-\kappa_A t/2}\Big\{\cos(\kappa_A t/2) + \sin(\kappa_A t/2)\Big\}. \tag{12}$$

From the above solution, it is clear that:

1. For $t < 0$, $A^{\text{out}}_g = i\sqrt{\kappa_a}e^{\kappa_a t/2}\theta(-t) = -A^{\text{out}}_e$, which indicates the $\pi$ phase-shift between the output signals when the qubit is in the ground and excited state.

2. For $t > 0$, $A^{\text{out}}_g = \sqrt{\kappa_a}\theta(t)e^{-\kappa_A t/2}e^{i\kappa_A t/2}(1+i) = A^{\text{out}*}_e$.

To find the information content of these pulses, we integrate $|A_g^{\text{out}}|^2$ and $|A_e^{\text{out}}|^2$.

Note that:

$$\int_{-\infty}^{0} |A_g^{\text{out}}|^2 dt = \int_{-\infty}^{0} |A_e^{\text{out}}|^2 dt = 1, \tag{13}$$

$$\int_{0}^{\infty} |A_g^{\text{out}}|^2 dt = \int_{0}^{\infty} |A_e^{\text{out}}|^2 dt = 2\frac{\kappa_a}{\kappa_A} \simeq 0 \text{ for } \kappa_{\text{a}} \ll \kappa_{\text{A}}. \tag{14}$$

So, for the choice of separation of time-scale, effectively, no photons come out for $t > 0$ and we can treat the output pulse to be a rising exponential wave packet with temporal profile: $\pm i\sqrt{\kappa_a} e^{\kappa_a t/2}\theta(-t)$, where $\pm$ depends on the state of the qubit being in $|g\rangle$ or $|e\rangle$. Numerical simulations have confirmed this result.

Based on the above computation, we can infer the loss of coherence due to the photons coming out for $t > 0$. This loss is can be computed to be $1 - e^{-|\alpha_0|^2 2\kappa_a/\kappa_A(1-|K|)}$, where $K$ is the overlap between the temporal profiles $A_g^{\text{out}}$ and $A_e^{\text{out}}$ for $t > 0$ and $\alpha_0$ is the coherent state amplitude incident on the cavity. For $\kappa_a \ll \kappa_A$, $|K| \to 1$ implying no loss of coherence.

To summarize our results, we have shown that a resonant, rising exponential pulse $\sqrt{\kappa_a} e^{\kappa_a t/2}\theta(-t)$ at the input of mode $A$ does indeed give rise to as output a rising exponential pulse $\pm i\sqrt{\kappa_a} e^{\kappa_a t/2}\theta(-t)$ in the $\kappa_a \ll \kappa_A$ regime, where the phase-shift of the reflected signal depends on the state of the qubit.

Note that the phase-shift was calculated in the continuous-wave case and experimentally demonstrated in [1]. Identical set of analysis can be performed for the interaction of the ancilla signal b with Bob's qubit.

## JOSEPHSON FOUR WAVE MIXER

The Josephson Four Wave Mixer (JFWM) consists of four identical Josephson junctions arranged as shown in Fig. 2. For the purposes of this work, we will operate with a bias currrent lower than the critical current $I_0$, when the Josephson junctions behave as pure nonlinear inductors, with nonlinear inductance given by: $L_J = \varphi_0/(I_0 \cos\delta)$, where $\delta$ is the gauge-invariant phase of the junction and $\varphi_0 = \hbar/(2e)$ is the reduced flux quantum. We define the node fluxes at nodes $x, y, z, w, u$ as :

$$V_i = \frac{d\Phi_i}{dt}, \qquad i = x, y, z, w, u, \tag{15}$$

where $V_i$ is potential at the node $i$. There are five normal modes of the JFWM, denoted by $\Phi_a, \Phi_b, \Phi_c, \Phi_d, \Phi_e$, described below:

$$\Phi_a = \Phi_x + \Phi_y - \Phi_z - \Phi_w, \tag{16}$$
$$\Phi_b = \Phi_x - \Phi_y - \Phi_z + \Phi_w, \tag{17}$$
$$\Phi_c = \Phi_x - \Phi_y + \Phi_z - \Phi_w, \tag{18}$$
$$\Phi_d = \Phi_x + \Phi_y + \Phi_z + \Phi_w - 4\Phi_u \text{ and} \tag{19}$$
$$\Phi_e = \Phi_x + \Phi_y + \Phi_z + \Phi_w + \Phi_u. \tag{20}$$

Out of these five modes, four $(\Phi_a, \Phi_b, \Phi_c, \Phi_d)$ participate in a nonlinear mode mixing, while the fifth $(\Phi_e)$ remain decoupled from the rest.

The Hamiltonian of the JFWM (denoted by $\mathbf{H}_{\text{JFWM}}$) is the sum of the Hamiltonian of each junction: $-E_J \cos\delta$, where $\delta$ is the gauge-invariant phase of the junction. Hence,

$$\mathbf{H}_{\text{JFWM}} = -E_J\Big(\cos\frac{\Phi_x - \Phi_u}{\varphi_0} + \cos\frac{\Phi_y - \Phi_u}{\varphi_0} + \cos\frac{\Phi_z - \Phi_u}{\varphi_0} + \cos\frac{\Phi_w - \Phi_u}{\varphi_0}\Big) \tag{21}$$

where $E_J = \varphi_0 I_0$ is the junction energy. Eq. (21) can be rewritten in terms of the normal modes of the JFWM as:

$$\mathbf{H}_{\text{JFWM}} = -4E_J \cos\frac{\Phi_a}{4\varphi_0}\cos\frac{\Phi_b}{4\varphi_0}\cos\frac{\Phi_c}{4\varphi_0}\cos\frac{\Phi_d}{4\varphi_0} + 4E_J \sin\frac{\Phi_a}{4\varphi_0}\sin\frac{\Phi_b}{4\varphi_0}\sin\frac{\Phi_c}{4\varphi_0}\sin\frac{\Phi_d}{4\varphi_0}. \tag{22}$$

For mode intensities $\Phi_a, \Phi_b, \Phi_c, \Phi_d \ll \varphi_0$, we can ignore terms of order higher than four in $\mathbf{H}_{\text{JFWM}}$, leading to:

$$\begin{aligned}\mathbf{H}_{\text{JFWM}} = -4E_J + \frac{E_J}{8\varphi_0^2}(\Phi_a^2 + \Phi_b^2 + \Phi_c^2 + \Phi_d^2) - \frac{E_J}{1536\varphi_0^4}(\Phi_a^4 + \Phi_b^4 + \Phi_c^4 + \Phi_d^4 + 6\Phi_a^2\Phi_b^2 + 6\Phi_a^2\Phi_c^2 \\ +6\Phi_a^2\Phi_d^2 + 6\Phi_b^2\Phi_c^2 + 6\Phi_b^2\Phi_d^2 + 6\Phi_c^2\Phi_d^2) + \frac{E_J}{64\varphi_0^4}\Phi_a\Phi_b\Phi_c\Phi_d.\end{aligned} \tag{23}$$

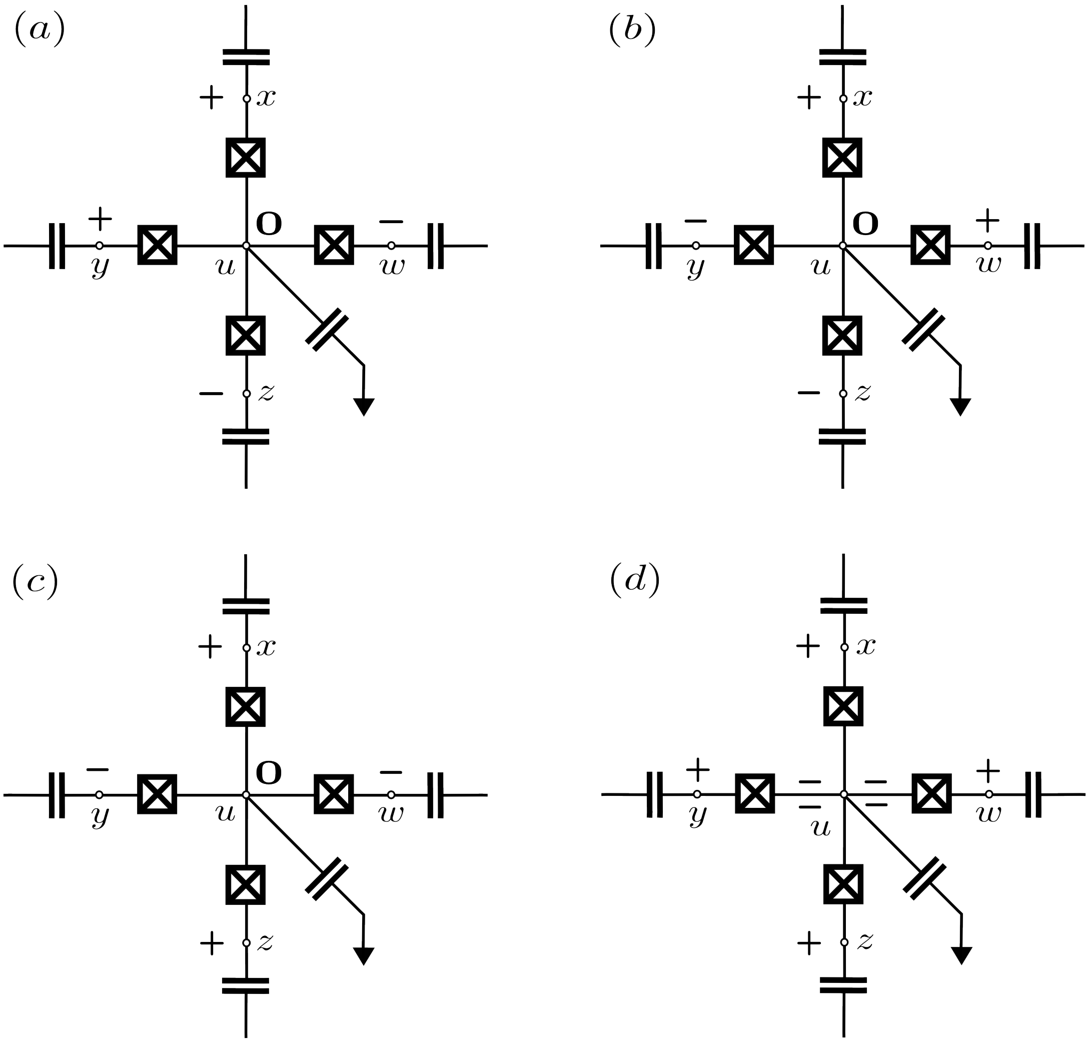


FIG. 2. The Josephson Four Wave Mixer (JFWM) has four nominally identical Josephson junctions and has four mutually orthogonal normal (electrical) modes, shown in (a), (b), (c) and (d). Modes (a), (b) and (c) respectively correspond to the ancilla signal a, ancilla signal b and parity signal c modes and (d) corresponds to the stiff, off-resonant pump. A fifth mode remains decoupled from the rest and is not shown here for brevity. The Josephson nonlinearity, together with the off-resonant pump, gives rise to the desired three-wave interaction given by $\mathbf{H}_{\text{int}}$.

We see that apart from the desired four wave mixing term: $\Phi_a\Phi_b\Phi_c\Phi_d$, the Hamiltonian has terms quadratic in mode amplitudes, which lead to frequency renormalization and other quartic terms which lead to self and cross Kerr nonlinearities. The three modes $\Phi_a, \Phi_b$ and $\Phi_c$ correspond to the ancilla signal a, ancilla signal b and parity signal modes, while $\Phi_d$ corresponds to a stiff, off-resonant pump. The pump enables the four-wave mixing term to be the dominant fourth order interaction term over the Kerr nonlinearities (neglected in subsequent analysis). In terms of the creation and annihilation operators for these modes, we can write:

$$\mathbf{\Phi_i} = \Phi_i^0(\mathbf{i} + \mathbf{i}^\dagger),\ i = a, b, c, d \text{ and } \Phi_{\rm i}^0 = \sqrt{\langle 0|\mathbf{\Phi_i}^2|0\rangle} \tag{24}$$

is the zero point fluctuation of the flux. The JFWM Hamiltonian can be rewritten as:

$$\mathbf{H}_{\text{JFWM}} = \hbar\omega_a\mathbf{a}^\dagger\mathbf{a} + \hbar\omega_b\mathbf{b}^\dagger\mathbf{b} + \hbar\omega_c\mathbf{c}^\dagger\mathbf{c} + \hbar\omega_d\mathbf{d}^\dagger\mathbf{d} + \hbar g_4(\mathbf{a}+\mathbf{a}^\dagger)(\mathbf{b}+\mathbf{b}^\dagger)(\mathbf{c}+\mathbf{c}^\dagger)(\mathbf{d}+\mathbf{d}^\dagger), \tag{25}$$

where $\omega_a, \omega_b, \omega_c, \omega_d$ are the renormalized frequencies of the modes $\mathbf{a}, \mathbf{b}, \mathbf{c}, \mathbf{d}$ and $g_4$ is the effective four-wave interaction strength. The pump frequency is chosen to be:

$$\omega_d = \omega_c - \omega_a - \omega_b, \tag{26}$$

which leads under rotating wave approximation (RWA) to:

$$\mathbf{H}_{\rm JFWM} = \hbar\omega_a \mathbf{a}^\dagger\mathbf{a} + \hbar\omega_b \mathbf{b}^\dagger\mathbf{b} + \hbar\omega_c \mathbf{c}^\dagger\mathbf{c} + \hbar\omega_d \mathbf{d}^\dagger\mathbf{d} + \hbar g_4 \mathbf{a}\mathbf{b}\mathbf{c}^\dagger\mathbf{d} + \text{h.c.} \tag{27}$$

The stiff, off-resonant pump gives rise to an effective three-wave interaction between the modes $\mathbf{a}, \mathbf{b}$ and $\mathbf{c}$ with a tunable coupling $g$, which depends on the pump strength. The leads to an effective Hamiltonian of the JFWM as:

$$\begin{aligned}\mathbf{H}_{\rm JFWM} &= \hbar\omega_a \mathbf{a}^\dagger\mathbf{a} + \hbar\omega_b \mathbf{b}^\dagger\mathbf{b} + \hbar\omega_c \mathbf{c}^\dagger\mathbf{c} + \mathbf{H}_{\rm int}, \\ \mathbf{H}_{\rm int} &= i\hbar g \mathbf{a}\mathbf{b}\mathbf{c}^\dagger + \text{h.c.}\end{aligned} \tag{28}$$

## QUASI-STEADY STATE COMPUTATION UNDER $\mathcal{D}(\mathbf{ab})$

The low-Q nature of the mode $\mathbf{c}$, together with the interaction Hamiltonian $\mathbf{H}_{\rm int}$ (cf. Eq. (28)), gives rise to an effective coupled mode dissipation of the form $\mathcal{D}(\mathbf{ab})$ with a dissipation rate $\kappa_{\rm 2ph} = 4g^2/\kappa_c \gg \kappa_a, \kappa_b$ [2], where $\kappa_a, \kappa_b$ and $\kappa_c$ are the decay rates of the modes $\mathbf{a}, \mathbf{b}$ and $\mathbf{c}$ respectively.

### Even Manifold Computation

In this subsection, we will describe the computation for the even manifold. Our aim is to compute the steady-state of solution of the Lindblad equation [3–5]:

$$\frac{d\rho_e}{dt} = \kappa_{\rm 2ph}\mathcal{D}(\mathbf{ab})\rho_e, \tag{29}$$

with the initial state: $\rho_e(t=0) = |\psi_e\rangle\langle\psi_e|$, $|\psi_e\rangle = \frac{1}{\sqrt{2}}(|ee,\alpha,\alpha\rangle + |gg,-\alpha,-\alpha\rangle)$, where for simplicity, we have chosen $\alpha = \beta$. The resulting steady state, denoted by $\rho_e^{\rm qs}$ can be written as:

$$\rho_e^{\rm qs} = \frac{1}{2}\big(\rho_e^{{\rm qs}(1)}|ee\rangle\langle ee| + \rho_e^{{\rm qs}(2)}|gg\rangle\langle gg| + \rho_e^{{\rm qs}(3)}|ee\rangle\langle gg| + \rho_e^{{\rm qs}(4)}|gg\rangle\langle ee|\big), \tag{30}$$

where

$$\rho_e^{\mathrm{qs}(1)} = \sum_{n=0}^{\infty} e^{-2|\alpha|^2} I_n(2|\alpha|^2)|n,0\rangle\langle n,0| + \sum_{n=1}^{\infty} e^{-2|\alpha|^2} I_n(2|\alpha|^2)|0,n\rangle\langle 0,n|$$
$$+\sum_{n=0}^{\infty}\sum_{\mu=1}^{\infty} e^{-2|\alpha|^2} I_{n+\mu/2}(2|\alpha|^2)\frac{\Gamma(n+\mu/2+1)}{\sqrt{n!(n+\mu)!}}\big\{|n,0\rangle\langle n+\mu,0| + |0,n\rangle\langle 0,n+\mu| + \text{h.c.}\big\}$$
$$+\sum_{n=1}^{\infty}\sum_{\mu=1}^{\infty} e^{-2|\alpha|^2} I_{(n+\mu)/2}(2|\alpha|^2)\frac{\Gamma(n/2+\mu/2+1)}{\sqrt{n!\mu!}}\big\{|n,0\rangle\langle 0,\mu| + |0,\mu\rangle\langle n,0|\big\}, \tag{31}$$

$$\rho_e^{\mathrm{qs}(2)} = \sum_{n=0}^{\infty} e^{-2|\alpha|^2} I_n(2|\alpha|^2)|n,0\rangle\langle n,0| + \sum_{n=1}^{\infty} e^{-2|\alpha|^2} I_n(2|\alpha|^2)|0,n\rangle\langle 0,n|$$
$$+\sum_{n=0}^{\infty}\sum_{\mu=1}^{\infty} e^{-2|\alpha|^2} I_{n+\mu/2}(2|\alpha|^2)\frac{(-1)^{\mu}\Gamma(n+\mu/2+1)}{\sqrt{n!(n+\mu)!}}\big\{|n,0\rangle\langle n+\mu,0| + |0,n\rangle\langle 0,n+\mu| + \text{h.c.}\big\}$$
$$+\sum_{n=1}^{\infty}\sum_{\mu=1}^{\infty} e^{-2|\alpha|^2} I_{(n+\mu)/2}(2|\alpha|^2)\frac{(-1)^{n-\mu}\Gamma(n/2+\mu/2+1)}{\sqrt{n!\mu!}}\big\{|n,0\rangle\langle 0,\mu| + |0,\mu\rangle\langle n,0|\big\}, \tag{32}$$

$$\rho_e^{\mathrm{qs}(3)} = \sum_{n=0}^{\infty} e^{-2|\alpha|^2}(-1)^n I_n(2|\alpha|^2)|n,0\rangle\langle n,0| + \sum_{n=1}^{\infty} e^{-2|\alpha|^2}(-1)^n I_n(2|\alpha|^2)|0,n\rangle\langle 0,n|$$
$$+\sum_{n=0}^{\infty}\sum_{\mu=1}^{\infty} e^{-2|\alpha|^2} I_{n+\mu/2}(2|\alpha|^2)\frac{(-1)^{n}\Gamma(n+\mu/2+1)}{\sqrt{n!(n+\mu)!}}\big\{(-1)^{\mu}|n,0\rangle\langle n+\mu,0| + |n+\mu,0\rangle\langle n,0|$$
$$+(-1)^{\mu}|0,n\rangle\langle 0,n+\mu| + |0,n+\mu\rangle\langle 0,n|\big\}$$
$$+\sum_{n=1}^{\infty}\sum_{\mu=1}^{\infty} e^{-2|\alpha|^2} I_{(n+\mu)/2}(2|\alpha|^2)\frac{\Gamma(n/2+\mu/2+1)}{\sqrt{n!\mu!}}\big\{(-1)^{\mu}|n,0\rangle\langle 0,\mu| + (-1)^{n}|0,\mu\rangle\langle n,0|\big\}, \tag{33}$$

$$\rho_e^{\mathrm{qs}(4)} = \sum_{n=0}^{\infty} e^{-2|\alpha|^2}(-1)^n I_n(2|\alpha|^2)|n,0\rangle\langle n,0| + \sum_{n=1}^{\infty} e^{-2|\alpha|^2}(-1)^n I_n(2|\alpha|^2)|0,n\rangle\langle 0,n|$$
$$+\sum_{n=0}^{\infty}\sum_{\mu=1}^{\infty} e^{-2|\alpha|^2} I_{n+\mu/2}(2|\alpha|^2)\frac{(-1)^{n+\mu}\Gamma(n+\mu/2+1)}{\sqrt{n!(n+\mu)!}}\big\{(-1)^{\mu}|n,0\rangle\langle n+\mu,0| + |n+\mu,0\rangle\langle n,0|$$
$$+(-1)^{\mu}|0,n\rangle\langle 0,n+\mu| + |0,n+\mu\rangle\langle 0,n|\big\}$$
$$+\sum_{n=1}^{\infty}\sum_{\mu=1}^{\infty} e^{-2|\alpha|^2} I_{(n+\mu)/2}(2|\alpha|^2)\frac{\Gamma(n/2+\mu/2+1)}{\sqrt{n!\mu!}}\big\{(-1)^{n}|n,0\rangle\langle 0,\mu| + (-1)^{\mu}|0,\mu\rangle\langle n,0|\big\}. \tag{34}$$

Here $I_n$ are the modified Bessel functions of the first kind of order $n$.

**Odd Manifold Computation**

In this subsection, we will describe the computation for the odd manifold. Our aim is to compute the steady-state of solution of the Lindblad equation:

$$\frac{d\rho_o}{dt} = \kappa_{2\mathrm{ph}}\mathcal{D}(\mathbf{ab})\rho_o, \tag{35}$$

with the initial state: $\rho_o(t=0) = |\psi_o\rangle\langle\psi_o|$, $|\psi_o\rangle = \frac{1}{\sqrt{2}}(|eg,\alpha,-\alpha\rangle + |ge,-\alpha,\alpha\rangle)$, again choosing $\alpha=\beta$ for simplicity. The resulting steady state, denoted by $\rho_e^{\mathrm{qs}}$ can be written as:

$$\rho_o^{\mathrm{qs}} = \frac{1}{2}\big(\rho_o^{\mathrm{qs}(1)}|eg\rangle\langle eg| + \rho_o^{\mathrm{qs}(2)}|ge\rangle\langle ge| + \rho_o^{\mathrm{qs}(3)}|eg\rangle\langle ge| + \rho_o^{\mathrm{qs}(4)}|ge\rangle\langle eg|\big), \tag{36}$$

where

$$\rho_o^{\mathrm{qs}(1)} = \sum_{n=0}^{\infty} e^{-2|\alpha|^2} I_n(2|\alpha|^2)|n,0\rangle\langle n,0| + \sum_{n=1}^{\infty} e^{-2|\alpha|^2} I_n(2|\alpha|^2)|0,n\rangle\langle 0,n|$$
$$+\sum_{n=0}^{\infty}\sum_{\mu=1}^{\infty} e^{-2|\alpha|^2} I_{n+\mu/2}(2|\alpha|^2)\frac{\Gamma(n+\mu/2+1)}{\sqrt{n!(n+\mu)!}}\big\{|n,0\rangle\langle n+\mu,0| + (-1)^{\mu}|0,n\rangle\langle 0,n+\mu| + \mathrm{h.c.}\big\}$$
$$+\sum_{n=1}^{\infty}\sum_{\mu=1}^{\infty} e^{-2|\alpha|^2} I_{(n+\mu)/2}(2|\alpha|^2)\frac{(-1)^{\mu}\Gamma(n/2+\mu/2+1)}{\sqrt{n!\mu!}}\big\{|n,0\rangle\langle 0,\mu| + |0,\mu\rangle\langle n,0|\big\}, \tag{37}$$

$$\rho_o^{\mathrm{qs}(2)} = \sum_{n=0}^{\infty} e^{-2|\alpha|^2} I_n(2|\alpha|^2)|n,0\rangle\langle n,0| + \sum_{n=1}^{\infty} e^{-2|\alpha|^2} I_n(2|\alpha|^2)|0,n\rangle\langle 0,n|$$
$$+\sum_{n=0}^{\infty}\sum_{\mu=1}^{\infty} e^{-2|\alpha|^2} I_{n+\mu/2}(2|\alpha|^2)\frac{\Gamma(n+\mu/2+1)}{\sqrt{n!(n+\mu)!}}\big\{(-1)^{\mu}|n,0\rangle\langle n+\mu,0| + |0,n\rangle\langle 0,n+\mu| + \mathrm{h.c.}\big\}$$
$$+\sum_{n=1}^{\infty}\sum_{\mu=1}^{\infty} e^{-2|\alpha|^2} I_{(n+\mu)/2}(2|\alpha|^2)\frac{(-1)^{n}\Gamma(n/2+\mu/2+1)}{\sqrt{n!\mu!}}\big\{|n,0\rangle\langle 0,\mu| + |0,\mu\rangle\langle n,0|\big\}, \tag{38}$$

$$\rho_o^{\mathrm{qs}(3)} = \sum_{n=0}^{\infty} e^{-2|\alpha|^2}(-1)^n I_n(2|\alpha|^2)|n,0\rangle\langle n,0| + \sum_{n=1}^{\infty} e^{-2|\alpha|^2}(-1)^n I_n(2|\alpha|^2)|0,n\rangle\langle 0,n|$$
$$+\sum_{n=0}^{\infty}\sum_{\mu=1}^{\infty} e^{-2|\alpha|^2} I_{n+\mu/2}(2|\alpha|^2)\frac{(-1)^{n}\Gamma(n+\mu/2+1)}{\sqrt{n!(n+\mu)!}}\big\{(-1)^{\mu}|n,0\rangle\langle n+\mu,0| + |n+\mu,0\rangle\langle n,0|$$
$$+|0,n\rangle\langle 0,n+\mu| + (-1)^{\mu}|0,n+\mu\rangle\langle 0,n|\big\}$$
$$+\sum_{n=1}^{\infty}\sum_{\mu=1}^{\infty} e^{-2|\alpha|^2} I_{(n+\mu)/2}(2|\alpha|^2)\frac{\Gamma(n/2+\mu/2+1)}{\sqrt{n!\mu!}}\big\{|n,0\rangle\langle 0,\mu| + (-1)^{n-\mu}|0,\mu\rangle\langle n,0|\big\}, \tag{39}$$

$$\rho_o^{\mathrm{qs}(4)} = \sum_{n=0}^{\infty} e^{-2|\alpha|^2}(-1)^n I_n(2|\alpha|^2)|n,0\rangle\langle n,0| + \sum_{n=1}^{\infty} e^{-2|\alpha|^2}(-1)^n I_n(2|\alpha|^2)|0,n\rangle\langle 0,n|$$
$$+\sum_{n=0}^{\infty}\sum_{\mu=1}^{\infty} e^{-2|\alpha|^2} I_{n+\mu/2}(2|\alpha|^2)\frac{(-1)^{n+\mu}\Gamma(n+\mu/2+1)}{\sqrt{n!(n+\mu)!}}\big\{(-1)^{\mu}|n,0\rangle\langle n+\mu,0| + |n+\mu,0\rangle\langle n,0|$$
$$+|0,n\rangle\langle 0,n+\mu| + (-1)^{\mu}|0,n+\mu\rangle\langle 0,n|\big\}$$
$$+\sum_{n=1}^{\infty}\sum_{\mu=1}^{\infty} e^{-2|\alpha|^2} I_{(n+\mu)/2}(2|\alpha|^2)\frac{\Gamma(n/2+\mu/2+1)}{\sqrt{n!\mu!}}\big\{(-1)^{n-\mu}|n,0\rangle\langle 0,\mu| + |0,\mu\rangle\langle n,0|\big\}. \tag{40}$$

## EVEN MANIFOLD COMPUTATION OF QUBIT STATE AFTER HOMODYNE DETECTION AT $\mathrm{HD}_a$ AND $\mathrm{HD}_b$

### X Measurement

For the detection of X quadratures of the modes **a** and **b**, the homodyne spectrum can be modeled by the projective measurement operators of the form $\mathcal{M}_X = |x_a, x_b\rangle\langle x_a, x_b|$, where $x_a, x_b$ are the outcomes of the integrated homodyne current at $\mathrm{HD_a}$ and $\mathrm{HD_b}$. The post-measurement state of the system is denoted by:

$$\rho_e^M = \frac{\mathcal{M}_X \rho_e^{\mathrm{qs}} \mathcal{M}_X^{\dagger}}{\mathrm{Tr}\big[\mathcal{M}_{\mathrm{X}} \rho_{\mathrm{e}}^{\mathrm{qs}} \mathcal{M}_{\mathrm{X}}^{\dagger}\big]} \tag{41}$$

and the final qubit state can be computed from Eq. (41) by tracing out the modes **a** and **b**. We use the following definition of the wavefunction of a Fock state in the position basis [6]:

$$\langle x|n\rangle = \left(\frac{2}{\pi}\right)^{1/4} \frac{1}{\sqrt{2^n n!}} e^{-x^2} H_n(x\sqrt{2}), \tag{42}$$

where $H_n$ are Hermite polynomials of order $n$. Using results obtained in the previous section and omitting a few lines of algebra, the post-measurement qubit state can be written as:

$$\rho_q(x_a,x_b) = \frac{1}{\lambda_1(x_a,x_b)+\lambda_2(x_a,x_b)}\Big(\lambda_1(x_a,x_b)|ee\rangle\langle ee| + \lambda_2(x_a,x_b)|gg\rangle\langle gg| + \lambda_3(x_a,x_b)|ee\rangle\langle gg| + \lambda_4(x_a,x_b)|gg\rangle\langle ee|\Big), \tag{43}$$

where

$$\begin{aligned}\lambda_1(x_a,x_b) = {}& \frac{2}{\pi}e^{-2(x_a^2+x_b^2)}e^{-2|\alpha|^2}\Big[\sum_{n=0}^{\infty}\frac{I_n(2|\alpha|^2)}{2^n n!}H_n(x_a\sqrt{2})^2 + \sum_{n=1}^{\infty}\frac{I_n(2|\alpha|^2)}{2^n n!}H_n(x_b\sqrt{2})^2 \\ & +2\sum_{n=0}^{\infty}\sum_{\mu=1}^{\infty}I_{n+\mu/2}(2|\alpha|^2)\frac{\Gamma(n+\mu/2+1)}{n!(n+\mu)!2^{n+\mu/2}}\Big\{H_n(x_a\sqrt{2})H_{n+\mu}(x_a\sqrt{2}) + H_n(x_b\sqrt{2})H_{n+\mu}(x_b\sqrt{2})\Big\} \\ & +2\sum_{n=1}^{\infty}\sum_{\mu=1}^{\infty}I_{(n+\mu)/2}(2|\alpha|^2)\frac{\Gamma(n/2+\mu/2+1)}{n!\mu!2^{(n+\mu)/2}}H_n(x_a\sqrt{2})H_\mu(x_b\sqrt{2})\Big],\end{aligned} \tag{44}$$

$$\begin{aligned}\lambda_2(x_a,x_b) = {}& \frac{2}{\pi}e^{-2(x_a^2+x_b^2)}e^{-2|\alpha|^2}\Big[\sum_{n=0}^{\infty}\frac{I_n(2|\alpha|^2)}{2^n n!}H_n(x_a\sqrt{2})^2 + \sum_{n=1}^{\infty}\frac{I_n(2|\alpha|^2)}{2^n n!}H_n(x_b\sqrt{2})^2 \\ & +2\sum_{n=0}^{\infty}\sum_{\mu=1}^{\infty}I_{n+\mu/2}(2|\alpha|^2)\frac{(-1)^\mu\Gamma(n+\mu/2+1)}{n!(n+\mu)!2^{n+\mu/2}}\Big\{H_n(x_a\sqrt{2})H_{n+\mu}(x_a\sqrt{2}) + H_n(x_b\sqrt{2})H_{n+\mu}(x_b\sqrt{2})\Big\} \\ & +2\sum_{n=1}^{\infty}\sum_{\mu=1}^{\infty}I_{(n+\mu)/2}(2|\alpha|^2)\frac{(-1)^{n-\mu}\Gamma(n/2+\mu/2+1)}{n!\mu!2^{(n+\mu)/2}}H_n(x_a\sqrt{2})H_\mu(x_b\sqrt{2})\Big],\end{aligned} \tag{45}$$

$$\begin{aligned}\lambda_3(x_a,x_b) = {}& \frac{2}{\pi}e^{-2(x_a^2+x_b^2)}e^{-2|\alpha|^2}\Big[\sum_{n=0}^{\infty}(-1)^n\frac{I_n(2|\alpha|^2)}{2^n n!}H_n(x_a\sqrt{2})^2 + \sum_{n=1}^{\infty}(-1)^n\frac{I_n(2|\alpha|^2)}{2^n n!}H_n(x_b\sqrt{2})^2 \\ & +\sum_{n=0}^{\infty}\sum_{\mu=1}^{\infty}I_{n+\mu/2}(2|\alpha|^2)\frac{\Gamma(n+\mu/2+1)}{n!(n+\mu)!2^{n+\mu/2}}(-1)^n\{(-1)^\mu+1\}\Big\{H_n(x_a\sqrt{2})H_{n+\mu}(x_a\sqrt{2}) + H_n(x_b\sqrt{2})H_{n+\mu}(x_b\sqrt{2})\Big\} \\ & +\sum_{n=1}^{\infty}\sum_{\mu=1}^{\infty}I_{(n+\mu)/2}(2|\alpha|^2)\frac{\Gamma(n/2+\mu/2+1)}{n!\mu!2^{(n+\mu)/2}}\{(-1)^n+(-1)^\mu\}H_n(x_a\sqrt{2})H_\mu(x_b\sqrt{2})\Big],\end{aligned} \tag{46}$$

$$\lambda_4(x_a,x_b) = \lambda_3(x_a,x_b)^*. \tag{47}$$

The probability distribution of the outcomes is denoted by:

$$P(x_a,x_b) = \frac{1}{2}\{\lambda_1(x_a,x_b)+\lambda_2(x_a,x_b)\} \tag{48}$$

and the overlap with the Bell-state $|\Phi^+\rangle$ is given by:

$$\langle\Phi^+|\rho_q(x_a,x_b)|\Phi^+\rangle = \frac{1}{2(\lambda_1(x_a,x_b)+\lambda_2(x_a,x_b))}\big\{\lambda_1(x_a,x_b)+\lambda_2(x_a,x_b)+\lambda_3(x_a,x_b)+\lambda_4(x_a,x_b)\big\}. \tag{49}$$

These are evaluated for $\alpha = 0.75$ in the main text.

### Y Measurement

In this case, $\mathcal{M}_X \to \mathcal{M}_Y = |y_a,y_b\rangle\langle y_a,y_b|$. We use the following definition of the wavefunction of a Fock state in the momentum basis:

$$\langle y|n\rangle = \Big(\frac{2}{\pi}\Big)^{1/4}\frac{(-i)^n}{\sqrt{2^n n!}}e^{-y^2}H_n(y\sqrt{2}), \tag{50}$$

where $H_n$ are Hermite polynomials of order $n$. Using results obtained in the previous section and omitting a few lines of algebra, the post-measurement qubit state can be written as:

$$\rho_q(y_a,y_b) = \frac{1}{\lambda_1(y_a,y_b)+\lambda_2(y_a,y_b)}\Big(\lambda_1(y_a,y_b)|ee\rangle\langle ee| + \lambda_2(y_a,y_b)|gg\rangle\langle gg| + \lambda_3(y_a,y_b)|ee\rangle\langle gg| + \lambda_4(y_a,y_b)|gg\rangle\langle ee|\Big), \tag{51}$$

where

$$\lambda_1(y_a,y_b) = \frac{2}{\pi}e^{-2(y_a^2+y_b^2)}e^{-2|\alpha|^2}\Big[\sum_{n=0}^{\infty}\frac{I_n(2|\alpha|^2)}{2^n n!}H_n(y_a\sqrt{2})^2 + \sum_{n=1}^{\infty}\frac{I_n(2|\alpha|^2)}{2^n n!}H_n(y_b\sqrt{2})^2$$
$$+\sum_{n=0}^{\infty}\sum_{\mu=1}^{\infty}I_{n+\mu/2}(2|\alpha|^2)\frac{\Gamma(n+\mu/2+1)}{n!(n+\mu)!2^{n+\mu/2}}\{i^\mu+(-i)^\mu\}\Big\{H_n(y_a\sqrt{2})H_{n+\mu}(y_a\sqrt{2})+H_n(y_b\sqrt{2})H_{n+\mu}(y_b\sqrt{2})\Big\}$$
$$+\sum_{n=1}^{\infty}\sum_{\mu=1}^{\infty}I_{(n+\mu)/2}(2|\alpha|^2)\frac{\Gamma(n/2+\mu/2+1)}{n!\mu!2^{(n+\mu)/2}}\{(-i)^n i^\mu + i^n(-i)^\mu\}H_n(y_a\sqrt{2})H_\mu(y_b\sqrt{2})\Big], \tag{52}$$

$$\lambda_2(y_a,y_b) = \frac{2}{\pi}e^{-2(y_a^2+y_b^2)}e^{-2|\alpha|^2}\Big[\sum_{n=0}^{\infty}\frac{I_n(2|\alpha|^2)}{2^n n!}H_n(y_a\sqrt{2})^2 + \sum_{n=1}^{\infty}\frac{I_n(2|\alpha|^2)}{2^n n!}H_n(y_b\sqrt{2})^2$$
$$+\sum_{n=0}^{\infty}\sum_{\mu=1}^{\infty}I_{n+\mu/2}(2|\alpha|^2)\frac{(-1)^\mu\Gamma(n+\mu/2+1)}{n!(n+\mu)!2^{n+\mu/2}}\{i^\mu+(-i)^\mu\}\Big\{H_n(y_a\sqrt{2})H_{n+\mu}(y_a\sqrt{2})+H_n(y_b\sqrt{2})H_{n+\mu}(y_b\sqrt{2})\Big\}$$
$$+\sum_{n=1}^{\infty}\sum_{\mu=1}^{\infty}I_{(n+\mu)/2}(2|\alpha|^2)\frac{(-1)^{n-\mu}\Gamma(n/2+\mu/2+1)}{n!\mu!2^{(n+\mu)/2}}\{(-i)^n i^\mu + i^n(-i)^\mu\}H_n(y_a\sqrt{2})H_\mu(y_b\sqrt{2})\Big], \tag{53}$$

$$\lambda_3(y_a,y_b) = \frac{2}{\pi}e^{-2(y_a^2+y_b^2)}e^{-2|\alpha|^2}\Big[\sum_{n=0}^{\infty}(-1)^n\frac{I_n(2|\alpha|^2)}{2^n n!}H_n(y_a\sqrt{2})^2 + \sum_{n=1}^{\infty}(-1)^n\frac{I_n(2|\alpha|^2)}{2^n n!}H_n(y_b\sqrt{2})^2$$
$$+2\sum_{n=0}^{\infty}\sum_{\mu=1}^{\infty}I_{n+\mu/2}(2|\alpha|^2)\frac{\Gamma(n+\mu/2+1)}{n!(n+\mu)!2^{n+\mu/2}}(-1)^n(-i)^\mu\Big\{H_n(y_a\sqrt{2})H_{n+\mu}(y_a\sqrt{2})+H_n(y_b\sqrt{2})H_{n+\mu}(y_b\sqrt{2})\Big\}$$
$$+2\sum_{n=1}^{\infty}\sum_{\mu=1}^{\infty}I_{(n+\mu)/2}(2|\alpha|^2)\frac{\Gamma(n/2+\mu/2+1)}{n!\mu!2^{(n+\mu)/2}}(-i)^{n+\mu}H_n(y_a\sqrt{2})H_\mu(y_b\sqrt{2})\Big], \tag{54}$$

$$\lambda_4(y_a,y_b) = \lambda_3(y_a,y_b)^*. \tag{55}$$

The probability distribution of the outcomes and overlap with the Bell-state $|\Phi^+\rangle$ can be computed as before.

## ODD MANIFOLD COMPUTATION OF QUBIT STATE AFTER HOMODYNE DETECTION AT $\mathrm{HD}_a$ AND $\mathrm{HD}_b$

A similar set of computation can be done for the odd manifold.

### X Measurements

In this case case, the post-measurement qubit state can similarly be defined as:

$$\rho_q(x_a,x_b) = \frac{1}{\lambda_1(x_a,x_b)+\lambda_2(x_a,x_b)}\Big(\lambda_1(x_a,x_b)|eg\rangle\langle eg| + \lambda_2(x_a,x_b)|ge\rangle\langle ge| + \lambda_3(x_a,x_b)|eg\rangle\langle ge| + \lambda_4(x_a,x_b)|ge\rangle\langle eg|\Big), \tag{56}$$

where

$$\lambda_1(x_a,x_b) = \frac{2}{\pi}e^{-2(x_a^2+x_b^2)}e^{-2|\alpha|^2}\Big[\sum_{n=0}^{\infty}\frac{I_n(2|\alpha|^2)}{2^n n!}H_n(x_a\sqrt{2})^2 + \sum_{n=1}^{\infty}\frac{I_n(2|\alpha|^2)}{2^n n!}H_n(x_b\sqrt{2})^2$$
$$+2\sum_{n=0}^{\infty}\sum_{\mu=1}^{\infty}I_{n+\mu/2}(2|\alpha|^2)\frac{\Gamma(n+\mu/2+1)}{n!(n+\mu)!2^{n+\mu/2}}\Big\{H_n(x_a\sqrt{2})H_{n+\mu}(x_a\sqrt{2}) + (-1)^{\mu}H_n(x_b\sqrt{2})H_{n+\mu}(x_b\sqrt{2})\Big\}$$
$$+2\sum_{n=1}^{\infty}\sum_{\mu=1}^{\infty}I_{(n+\mu)/2}(2|\alpha|^2)\frac{(-1)^{\mu}\Gamma(n/2+\mu/2+1)}{n!\mu!2^{(n+\mu)/2}}H_n(x_a\sqrt{2})H_{\mu}(x_b\sqrt{2})\Big], \quad (57)$$

$$\lambda_2(x_a,x_b) = \frac{2}{\pi}e^{-2(x_a^2+x_b^2)}e^{-2|\alpha|^2}\Big[\sum_{n=0}^{\infty}\frac{I_n(2|\alpha|^2)}{2^n n!}H_n(x_a\sqrt{2})^2 + \sum_{n=1}^{\infty}\frac{I_n(2|\alpha|^2)}{2^n n!}H_n(x_b\sqrt{2})^2$$
$$+2\sum_{n=0}^{\infty}\sum_{\mu=1}^{\infty}I_{n+\mu/2}(2|\alpha|^2)\frac{\Gamma(n+\mu/2+1)}{n!(n+\mu)!2^{n+\mu/2}}\Big\{(-1)^{\mu}H_n(x_a\sqrt{2})H_{n+\mu}(x_a\sqrt{2}) + H_n(x_b\sqrt{2})H_{n+\mu}(x_b\sqrt{2})\Big\}$$
$$+2\sum_{n=1}^{\infty}\sum_{\mu=1}^{\infty}I_{(n+\mu)/2}(2|\alpha|^2)\frac{(-1)^{n}\Gamma(n/2+\mu/2+1)}{n!\mu!2^{(n+\mu)/2}}H_n(x_a\sqrt{2})H_{\mu}(x_b\sqrt{2})\Big], \quad (58)$$

$$\lambda_3(x_a,x_b) = \frac{2}{\pi}e^{-2(x_a^2+x_b^2)}e^{-2|\alpha|^2}\Big[\sum_{n=0}^{\infty}(-1)^n\frac{I_n(2|\alpha|^2)}{2^n n!}H_n(x_a\sqrt{2})^2 + \sum_{n=1}^{\infty}(-1)^n\frac{I_n(2|\alpha|^2)}{2^n n!}H_n(x_b\sqrt{2})^2$$
$$+\sum_{n=0}^{\infty}\sum_{\mu=1}^{\infty}I_{n+\mu/2}(2|\alpha|^2)\frac{\Gamma(n+\mu/2+1)}{n!(n+\mu)!2^{n+\mu/2}}(-1)^n\big\{(-1)^{\mu}+1\big\}\Big\{H_n(x_a\sqrt{2})H_{n+\mu}(x_a\sqrt{2}) + H_n(x_b\sqrt{2})H_{n+\mu}(x_b\sqrt{2})\Big\}$$
$$+\sum_{n=1}^{\infty}\sum_{\mu=1}^{\infty}I_{(n+\mu)/2}(2|\alpha|^2)\frac{\Gamma(n/2+\mu/2+1)}{n!\mu!2^{(n+\mu)/2}}\big\{(-1)^{n-\mu}+1\big\}H_n(x_a\sqrt{2})H_{\mu}(x_b\sqrt{2})\Big], \quad (59)$$

$$\lambda_4(x_a,x_b) = \lambda_3(x_a,x_b)^*. \quad (60)$$

**Y Measurements**

In this case case, the post-measurement qubit state can similarly be defined as:

$$\rho_q(y_a,y_b) = \frac{1}{\lambda_1(y_a,y_b)+\lambda_2(y_a,y_b)}\Big(\lambda_1(y_a,y_b)|eg\rangle\langle eg| + \lambda_2(y_a,y_b)|ge\rangle\langle ge| + \lambda_3(y_a,y_b)|eg\rangle\langle ge| + \lambda_4(y_a,y_b)|ge\rangle\langle eg|\Big), \quad (61)$$

where

$$\lambda_1(y_a,y_b) = \frac{2}{\pi}e^{-2(y_a^2+y_b^2)}e^{-2|\alpha|^2}\Big[\sum_{n=0}^{\infty}\frac{I_n(2|\alpha|^2)}{2^n n!}H_n(y_a\sqrt{2})^2+\sum_{n=1}^{\infty}\frac{I_n(2|\alpha|^2)}{2^n n!}H_n(y_b\sqrt{2})^2$$
$$+\sum_{n=0}^{\infty}\sum_{\mu=1}^{\infty}I_{n+\mu/2}(2|\alpha|^2)\frac{\Gamma(n+\mu/2+1)}{n!(n+\mu)!2^{n+\mu/2}}\{i^\mu+(-i)^\mu\}\Big\{H_n(y_a\sqrt{2})H_{n+\mu}(y_a\sqrt{2})+(-1)^\mu H_n(y_b\sqrt{2})H_{n+\mu}(y_b\sqrt{2})\Big\}$$
$$+\sum_{n=1}^{\infty}\sum_{\mu=1}^{\infty}I_{(n+\mu)/2}(2|\alpha|^2)\frac{\Gamma(n/2+\mu/2+1)}{n!\mu!2^{(n+\mu)/2}}\{(-i)^n i^\mu+i^n(-i)^\mu\}(-1)^\mu H_n(y_a\sqrt{2})H_\mu(y_b\sqrt{2})\Big], \quad (62)$$

$$\lambda_2(y_a,y_b) = \frac{2}{\pi}e^{-2(y_a^2+y_b^2)}e^{-2|\alpha|^2}\Big[\sum_{n=0}^{\infty}\frac{I_n(2|\alpha|^2)}{2^n n!}H_n(y_a\sqrt{2})^2+\sum_{n=1}^{\infty}\frac{I_n(2|\alpha|^2)}{2^n n!}H_n(y_b\sqrt{2})^2$$
$$+\sum_{n=0}^{\infty}\sum_{\mu=1}^{\infty}I_{n+\mu/2}(2|\alpha|^2)\frac{(-1)^\mu\Gamma(n+\mu/2+1)}{n!(n+\mu)!2^{n+\mu/2}}\{i^\mu+(-i)^\mu\}\Big\{(-1)^\mu H_n(y_a\sqrt{2})H_{n+\mu}(y_a\sqrt{2})+H_n(y_b\sqrt{2})H_{n+\mu}(y_b\sqrt{2})\Big\}$$
$$+\sum_{n=1}^{\infty}\sum_{\mu=1}^{\infty}I_{(n+\mu)/2}(2|\alpha|^2)\frac{(-1)^\mu\Gamma(n/2+\mu/2+1)}{n!\mu!2^{(n+\mu)/2}}\{(-i)^n i^\mu+i^n(-i)^\mu\}H_n(y_a\sqrt{2})H_\mu(y_b\sqrt{2})\Big], \quad (63)$$

$$\lambda_3(y_a,y_b) = \frac{2}{\pi}e^{-2(y_a^2+y_b^2)}e^{-2|\alpha|^2}\Big[\sum_{n=0}^{\infty}(-1)^n\frac{I_n(2|\alpha|^2)}{2^n n!}H_n(y_a\sqrt{2})^2+\sum_{n=1}^{\infty}(-1)^n\frac{I_n(2|\alpha|^2)}{2^n n!}H_n(y_b\sqrt{2})^2$$
$$+\sum_{n=0}^{\infty}\sum_{\mu=1}^{\infty}I_{n+\mu/2}(2|\alpha|^2)\frac{\Gamma(n+\mu/2+1)}{n!(n+\mu)!2^{n+\mu/2}}(-1)^n\Big\{(1+(-1)^\mu)H_n(y_a\sqrt{2})H_{n+\mu}(y_a\sqrt{2})$$
$$+2i^\mu H_n(y_b\sqrt{2})H_{n+\mu}(y_b\sqrt{2})\Big\}+2\sum_{n=1}^{\infty}\sum_{\mu=1}^{\infty}I_{(n+\mu)/2}(2|\alpha|^2)\frac{\Gamma(n/2+\mu/2+1)}{n!\mu!2^{(n+\mu)/2}}(-i)^n i^\mu H_n(y_a\sqrt{2})H_\mu(y_b\sqrt{2})\Big], \quad (64)$$

$$\lambda_4(y_a,y_b) = \lambda_3(y_a,y_b)^*. \quad (65)$$

## COMPARISON OF ANALYTICAL SOLUTION WITH NUMERICAL SIMULATIONS

The analytical results shown above are performed approximating the stochastic evolution in step (II) of the protocol with a deterministic evolution. This deterministic evolution leads to the quasi-steady state solution $\rho^{\mathrm{qs}}_{e(o)}$ being impure, which results in the post-measurement qubit state $\rho_q$ being impure for a few outcomes. This is reflected in the concurrence shown in Fig. 3, which goes to zero for these outcomes. A full stochastic master equation simulation shows that these are artifacts of the approximation and are absent in the stochastic master equation simulation. Overlap of the qubit states obtained from stochastic master equation solution (denoted by $\rho_q^{\mathrm{SME}}$) with the analytical solutions (denoted by $\rho_q^{\mathrm{ana}}$) is shown in Fig. 3 for two cases: $\alpha=\beta=0.75$ and $\alpha=\beta=1$. In each of the cases, a sample of 500 trajectoriers are simulated. For most of the outcomes, the fidelity is well in excess of 90%, while for a certain number of outcomes it is lower and it is checked that these points correspond to the points of zero concurrence. The impurity grows as the $\alpha,\beta$ are increased and this restricts the validity of the analytical model to large $\alpha,\beta$.

* ananda.roy@yale.edu

[1] M. Hatridge, S. Shankar, M. Mirrahimi, F. Schackert, K. Geerlings, T. Brecht, K. M. Sliwa, B. Abdo, L. Frunzio, S. M. Girvin, R. J. Schoelkopf, and M. H. Devoret, Science **339**, 178 (2013), http://www.sciencemag.org/content/339/6116/178.full.pdf.
[2] H. Carmichael, *Statistical Methods in Quantum Optics 2: Non-Classical Fields*, Statistical Methods in Quantum Optics (Springer, 2007).
[3] H. D. Simaan and R. Loudon, Journal of Physics A: Mathematical and General **11**, 435 (1978).
[4] H. Simaan, Optics Communications **31**, 21 (1979).
[5] V. V. Albert and L. Jiang, Phys. Rev. A **89**, 022118 (2014).
[6] S. Haroche and J. M. Raimond, *Exploring the Quantum: Atoms, Cavities, and Photons* (Oxford Univ. Press, Oxford, 2006).

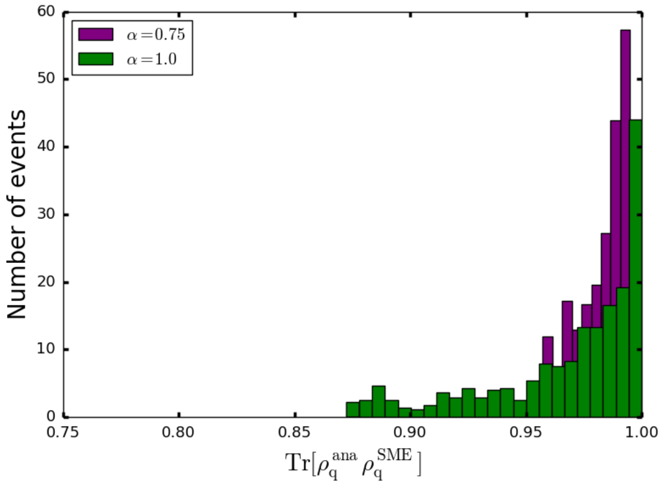


FIG. 3. Overlap of the qubit states obtained from analytical and stochastic master equation simulations for $\alpha = \beta = 0.75$ and $\alpha = \beta = 1$. In each of the cases, a sample of 500 trajectories are simulated. For $\alpha = \beta = 0.75$, the overlap between the qubit states obtained from the stochastic master equation simulation ($\rho_q^{\mathrm{SME}}$) and the corresponding analytical solution $\rho_q^{\mathrm{ana}}$ is more than 90%, indicating a strong overlap of the model with numerics. For $\alpha = \beta = 1$, we do see a few outcomes with lower fidelity, which correspond to the cases when the concurrence goes to zero.
